# Supplementary material for: Generalized Orthogonal de Bruijn and Kautz Sequences
Source: arXiv:2501.12921 source file (2025-02-22)
Supplement: Supplementary file 1 [file Appendix.tex]

%%%%%%
%% Appendix:
%% If needed a single appendix is created by
%%
%\appendix
%%
%% If several appendices are needed, then the command
%%
% \appendices
%%
%% in combination with further \section commands can be used.
%%%%%%
